# Supplementary material for: OFDM-based Waveforms for Joint Sensing and Communications Robust to Frequency Selective IQ Imbalance
Source: arXiv:2311.09746 source file (2023-11-16)
Supplement: Supplementary file 1 [file Appendix.tex]

\section{Derivation of the Relationship between CIR and ECIR}  \label{sec:Appendix_A}

This appendix analyzes the relation between the \ac{cir} $\ve{f}\in \mathbb{C}^{N_\ve{f}}$ and the \ac{ecir} $\ve{g}\in \mathbb{C}^{N_\text{a}}$ introduced in Sec.~\ref{sec:channel_model}. 

The \ac{ecir} $\ve{g}\in \mathbb{C}^{N_\text{a}}$ can be derived in vector representation from the \ac{ecfr} $\ve{h}\in \mathbb{C}^{N_\text{a}}$ according to \eqref{equ:Comm_OFDM_ECIR_002u}. Hence, the  $n$-th element of $\ve{g}$  is given by
\begin{align}
 \left[ \ve{g} \right]_{n} = \frac{1}{N_\text{a}} \sum_{k=0}^{N_\text{a}-1} \left[ \ve{h} \right]_{k} \, \mathrm{exp}\left(j2 \pi \frac{kn}{ N_\text{a}}\right) \hspace{5mm} \text{for} \, \, \, 0 \leq n < N_\text{a}. \label{equ:App_001}
\end{align}
The $k$-th element of $\ve{h}$, denoted as $\left[ \ve{h} \right]_{k}$, on the other hand can be obtained from the \ac{cfr} $\ve{p}\in \mathbb{C}^{N_\text{c}}$ according to
\begin{align}
 \left[ \ve{h} \right]_{k} = \left[ \ve{p} \right]_{\mu k} \hspace{5mm} \text{for} \, \, \, 0 \leq k < N_\text{a}. \label{equ:App_002}
\end{align}
By reformulating \eqref{equ:Comm_OFDM_ECIR_002o}, the scalars $\left[ \ve{p} \right]_{\mu k}$ can be identified to be
\begin{align}
 \left[ \ve{p} \right]_{\mu k} = \sum_{m=0}^{N_\ve{f}-1} \left[ \ve{f} \right]_{m} \, \mathrm{exp}\left(-j2 \pi \frac{ \mu km}{ N_\text{c}}\right) \hspace{5mm} \text{for} \, \, \, 0 \leq k < N_\text{a}. \label{equ:App_003}
\end{align}
Combining \eqref{equ:App_001}--\eqref{equ:App_003} allows for
\begin{align}
 \left[ \ve{g} \right]_{n} &={} \frac{1}{N_\text{a}} \sum_{k=0}^{N_\text{a}-1} \left( \sum_{m=0}^{N_\ve{f}-1} \left[ \ve{f} \right]_{m} \, \mathrm{exp}\left(-j2 \pi \frac{ \mu km}{ N_\text{c}}\right) \right)  \nonumber \\
 & \hspace{3mm} \cdot \, \mathrm{exp}\left(j2 \pi \frac{ kn}{ N_\text{a}}\right)  \label{equ:App_004} \\
 &={} \frac{1}{N_\text{a}} \sum_{k=0}^{N_\text{a}-1}  \sum_{m=0}^{N_\ve{f}-1} \left[ \ve{f} \right]_{m} \, \mathrm{exp}\left(j2 \pi k \left( \frac{ n}{ N_\text{a}}- \frac{ \mu m}{ N_\text{c}}\right) \right)   \label{equ:App_005} \\
  &={} \frac{1}{N_\text{a}} \sum_{m=0}^{N_\ve{f}-1} \left[ \ve{f} \right]_{m} \underbrace{ \left( \sum_{k=0}^{N_\text{a}-1}   \, \mathrm{exp}\left(j2 \pi k\left( \frac{ n}{ N_\text{a}}- \frac{ \mu m}{ N_\text{c}}\right) \right)  \right) }_{s(n,m)}  \label{equ:App_006} \\ 
  &={} \frac{1}{N_\text{a}} \sum_{m=0}^{N_\text{c}-1} \left[ \ve{f} \right]_{m} s(n,m).  \label{equ:App_007}
\end{align}
The scalar $s(n,m)\in \mathbb{C}$ depends on $\mu$, $N_\text{c}$, and $N_\text{a}$, and is analyzed for two cases. 

The first case is when $N_\text{c} / \mu = N_\text{a}$, for which $s(n,m)$ is a scaled Dirac delta function $s(n,m) = N_\text{a} \, \delta \left[ \left(n-m \right) \% N_\text{a} \right] $. Thus, it follows that the observed \ac{ecir} corresponds to 
\begin{align}
 \left[ \ve{g} \right]_{n} &={} \sum_{m=0}^{N_\ve{f}-1} \left[ \ve{f} \right]_{m} \delta \left[ \left(n-m \right) \% N_\text{a} \right]  \label{equ:App_008}
\end{align}
with $0 \leq n < N_\text{a}$. A further simplification is observed when $N_\ve{f} \leq N_\text{a}$, for which it holds that 
\begin{align}
 \left[ \ve{g} \right]_{n} &={}  \left[ \ve{f} \right]_{n}  \hspace{5mm} \text{for} \, \, \, 0 \leq n < N_\ve{f} \label{equ:App_009}
\end{align}
for $0 \leq n < N_\ve{f}$, and $\left[ \ve{g} \right]_{n} = 0$ for $N_\ve{f} \leq n < N_\text{a}$.
Thus, in this scenario, the \ac{ecir} is equivalent to the \ac{cir} zero-padded to a length of $N_\text{a}$.

The second case is when $N_\text{c} / \mu \neq N_\text{a}$, for which $s(n,m)$ is not a scaled Dirac delta function anymore. Then, the \ac{ecfr} $\ve{g}$ corresponds to the \ac{cir} $\ve{f}$ distorted by windowing effects, and can be derived via \eqref{equ:App_006}.
